# Supplementary material for: The explicit characterization of counterion dynamics around a flexible polyelectrolyte
Source: arXiv:2112.08848 source file (2021-12-16)
Supplement: Supplementary file 1 [file diffusion_SI__material.pdf]

# The explicit characterization of counterion dynamics around a flexible polyelectrolyte

Keerthi Radhakrishnan* and Sunil P Singh†
*Department of Physics,*
*Indian Institute Of Science Education and Research,*
*Bhopal 462 066, Madhya Pradesh, India*‡

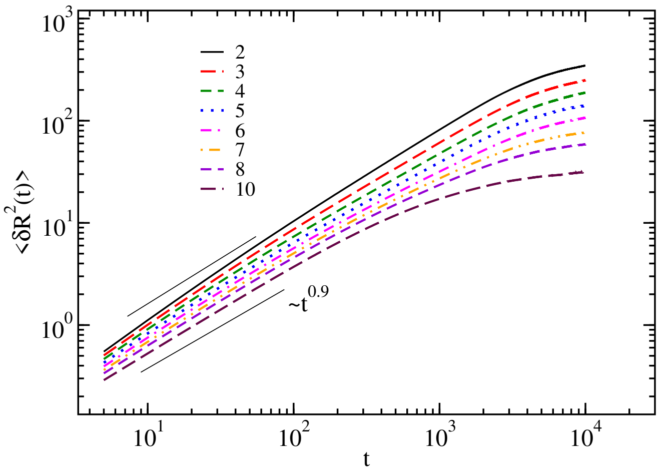


FIG. 1. The mean-square-displacement $< \delta R^2(t) >$ of the counterions as function of time for various electrostatic-interaction strength $\Gamma$ as indicated in the plot. At short times, ion excecutes effective diffusion $\langle \delta R^2 \rangle \sim t^\delta, \delta \approx 0.9$, followed by a transition to plateau regime. The pronounced influence of chain at large times can be substantiated from the plot as its observed that the crossover to the plateau roughly happens at timescales when a polymer diffuses its own size, $t_p = {R_g}^2/6D$. Like for $\Gamma$ 2 ($R_g \sim 9$) and 10($R_g \sim 4$), $t_p$ approx. 12000 and 1500, respectively.

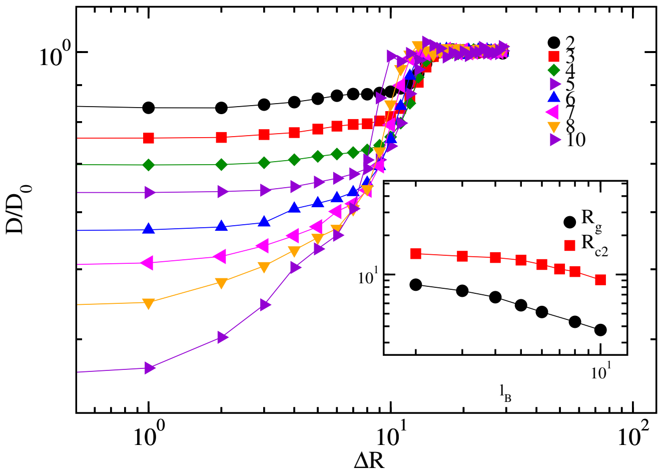


FIG. 2. The relative pair diffusion coefficient $D_R$ of the counterions w.r.t. COM as a function of the radial distance $R = |r - R_{cm}|$ for $N_m = 50$. Inset shows $R_g$ and $R_{c2}$ obtained from the main plot. For chain length $N = 50$ the polymer diffusivity is roughly 0.001 for $l_B = 2.0$ that is much smaller than the adsorbed ions diffusion.

## I. TEMPORAL EVOLUTION OF ION RELATIVE TO CHAIN

To get closer insights regarding the spatial evolution of ions w.r.t. the chain backbone, we tag a counterion and trace its nearest distance from the chain backbone over progressing time. This is elucidated in Fig. 3 Evidently, the trajectory indicates that for most of the time counterion stays tightly bound to the chain as $\rho \approx \sigma$ followed by occasional excursions represented by sharp peaks, where the counterion desorbs from the polymer surface. This can be also inferred from the distribution of ions shown in Fig.2 of the main manuscript. Further, the distance an ion traverses after desorption hardly extends beyond $2.5\sigma$. This is again because ion's navigation within the chain proximity is frequented with direct contacts with the fluctuating chain segments.

## II. ION RELAXATION MODES IN PE

The dielectric spectra of PEs seen in experiments consists of HF (in MHz range) and LF (in KHz range) relaxation mode, where the general consensus was that these primarily stems from the relaxation of uncondensed and condensed counterions, in addition to spectral contributions coming from the polarizability of the background solvent. A simplistic approach used to physically interpret these relaxation is to scale them in terms of ion's diffusivity $D_0$ following $\tau \sim \Delta^2/D_0$, to procure system relevant length scales ($\Delta$). In scaling theories for the PE solutions, where PE is seen as a linear chain of length L, the timescale associated with the condensed ion is given as $\tau \sim \frac{L^2}{D_0}$ and the free ion is given as $\tau \sim \frac{\zeta^2}{D_0}$ with $\zeta$ being the mean distance between PE chains.

Here, we leverage our access to the distinct length scales of ion association found around a flexible PE chain and varying ion diffusivity across regions to estimate associated ion timescales. For condensed counterions, possessing the lowest diffisivity over length scales of

* keerthirk@iiserb.ac.in
† spsingh@iiserb.ac.in
‡ spsingh@iiserb.ac.in; keerthirk@iiserb.ac.in

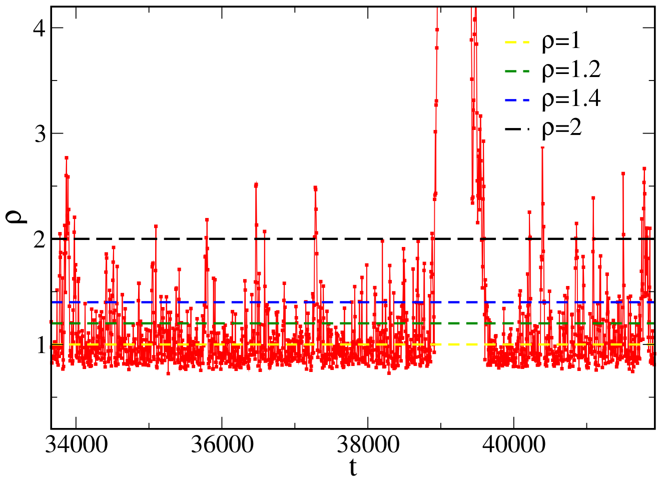


FIG. 3. Time evolution of a tagged counterion's nearest distance to the chain $\rho$, where dashed lines correspond for the minimum distance between the ion-chain duo $\rho_c = 1.0$ (yellow), 1.2 (green), 1.4 (blue), and 2.0 (black).

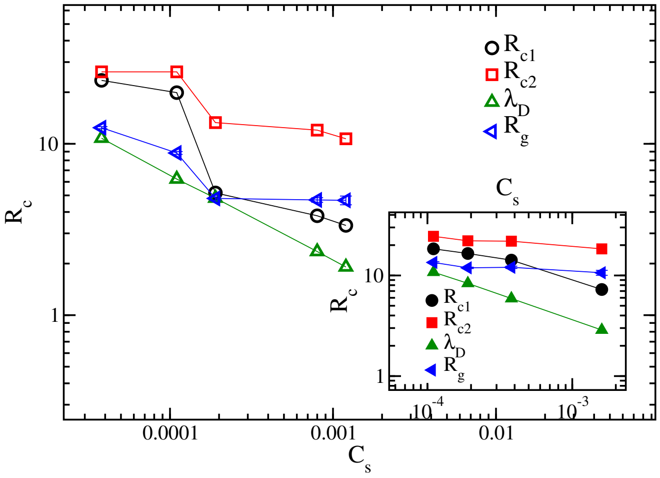


FIG. 4. Variation in $R_{c1}$, $R_{c2}$, $R_g$, and $\lambda_D$ (Debye length) with salt concentration for the case of divalent salt at $l_B = 3.0$ corresponding to $\Gamma = 6.0$.(Inset) Variation in $R_{c1}$, $R_{c2}$, $\lambda_D$, $R_g$ with salt concentration $C_s$ for monovalent salt at $l_B = 3.0$ which corresponds for $\Gamma = 3.0$.

roughly $R_g$, we get $\tau_c = \frac{R_{c1}{}^2}{D_R(0)}$, while, for the free ions we get $\tau_f = \frac{(L-R_{c2})^2}{D_0}$. Mapping our system's lowest timescale of ion diffusion in bulk i.e. $\tau_0 = \frac{\sigma^2}{D_0}$ to the diffusion scale of a typical particle of radius $a \sim 10^{-10}$m immersed in water of viscosity $\eta_w = 10^{-3} Kgm^{-1}s^{-1}$ i.e. $5 \times 10^{-12}$sec, we get the intrinsic timescale of the ion in real units. The mapped frequency modes acquired in real units is shown in Fig.5. Since, the timescales retrieved for both condensed and free ion here are within an order different and spans the MHz range (HF), it is safer to assert that the relaxation modes of these ions are not sufficient to account for the gap between HF (MHz) and the LF (KHz) modes. A confirmation of which is provided in recent works, where the LF mode with its ambiguous origin was attributed to the mean escape time of counterions from the PE surface.

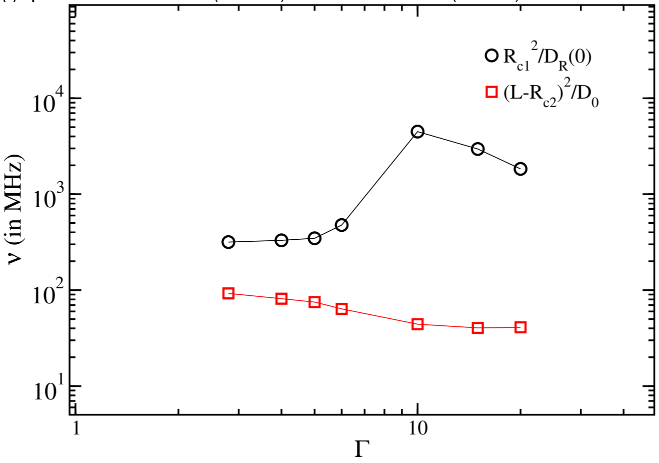


FIG. 5. Intrinsic relaxation modes associated with condensed counterions (bullets) and free ions (square) acquired in real units with ion timescale ($6\pi\eta_s a^3/K_BT = 5 \times 10^{-12}$ secs). Here, $\tau_c$ for condensed ion is defined $\tau_c = \frac{R_{c_1}{}^2}{D_R(0)}$ and $\tau_f$ for free ions is taken $\tau_f = \frac{(L-R_{c_2})^2}{D_0}$, where $R_{c_1}$ and $R_{c_2}$ demarcate bound and free ions around a flexible PE of chain length $N = 100$ as quantified in Fig.5-a in the manuscript. Note that $D_R(0)$ is effective diffusion of condensed ions.
